# Supplementary material for: Versatile Diffusion: Text, Images and Variations All in One Diffusion Model
Source: arXiv:2211.08332 source file (2024-01-11)
Supplement: Supplementary file 1 [file suppfig_vd_alt_0.tex]

\begin{figure}[t]
    \centering
    \includegraphics[width=0.76\textwidth]{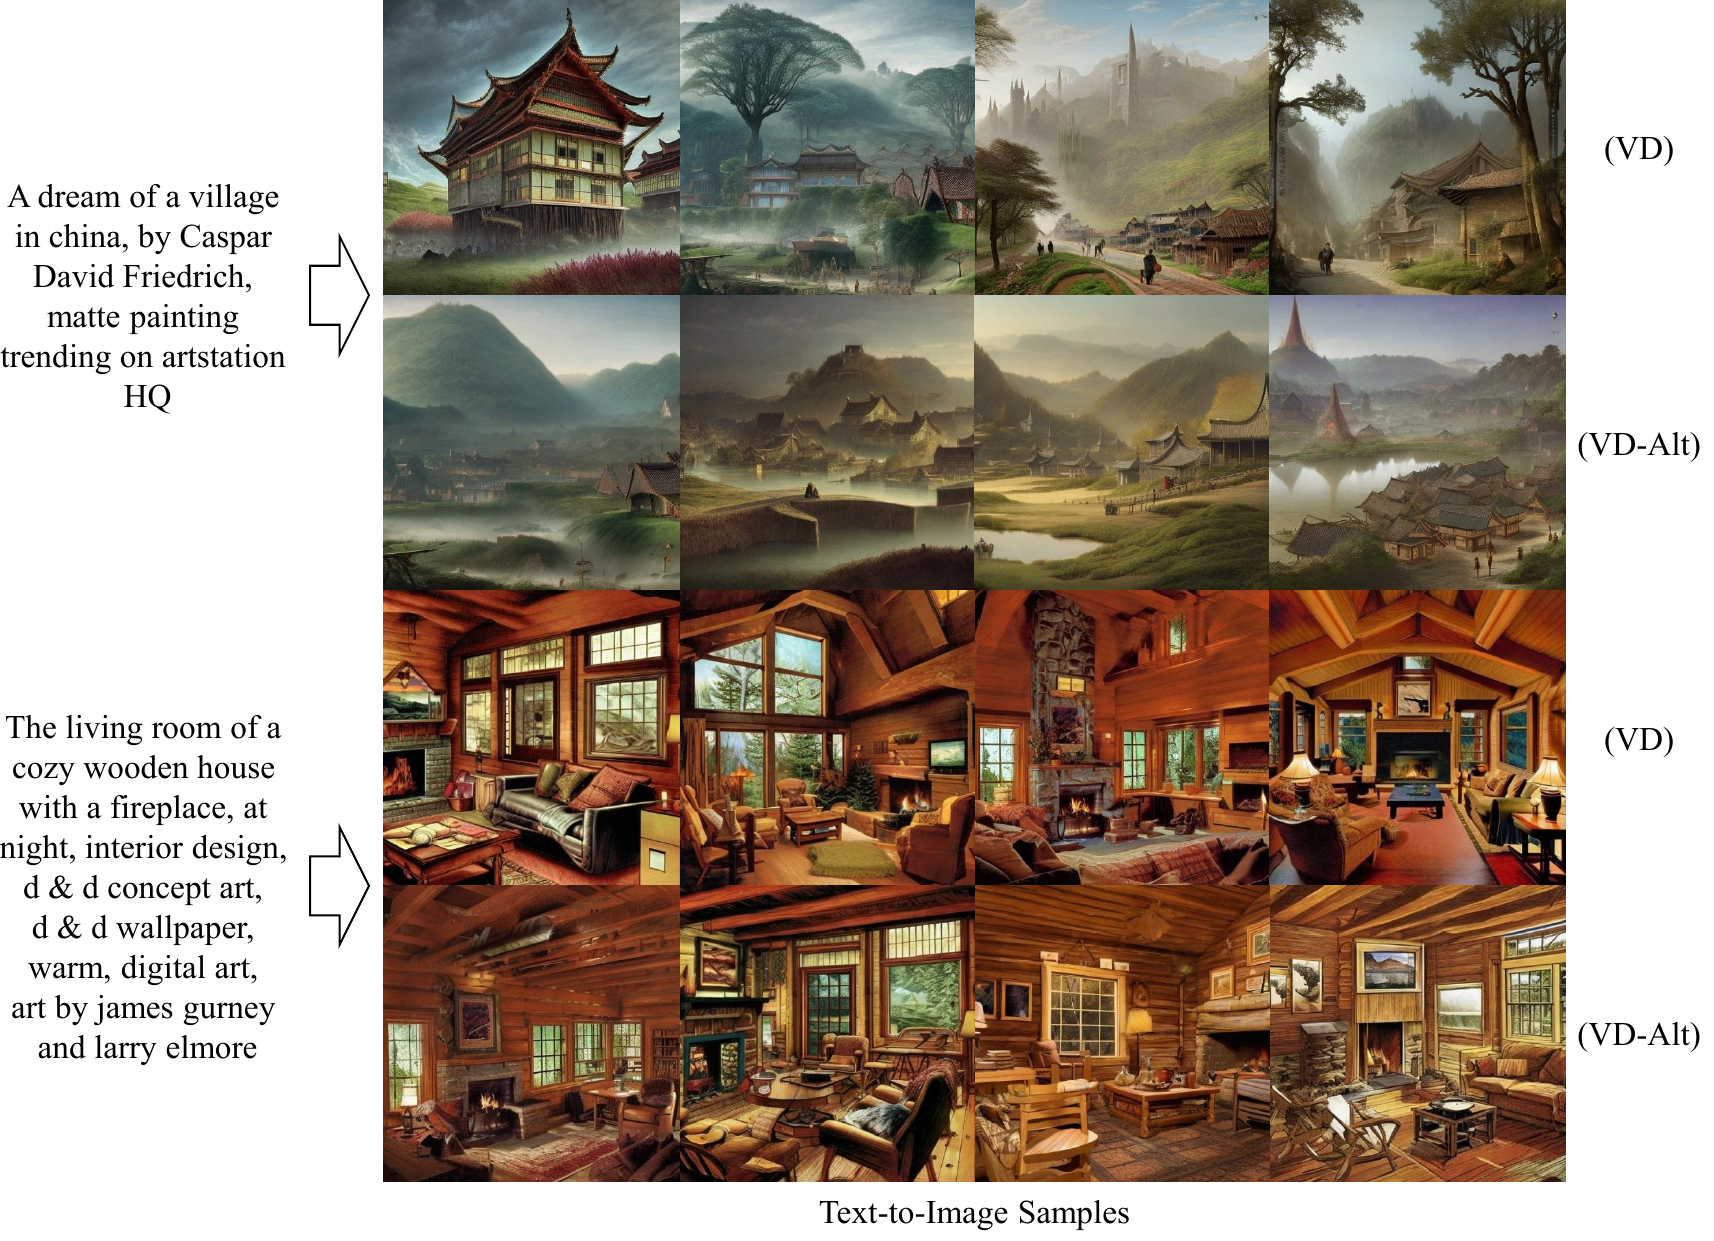}
    \caption{The qualitative comparison between VD and VD-Alt on text-to-image}
    \label{fig:supp_vd_alt_0}
\end{figure}
